# Supplementary material for: HOIGS: Human-Object Interaction Gaussian Splatting
Source: arXiv:2604.04016 source file (2026-04-05)
Supplement: Supplementary file 1 [file main_suppl.tex]

\begin{center}
\textbf{\large Supplementary Material \textit{for} \\ \vspace{2mm}
\large{``Expressive Whole-Body 3D Gaussian Avatar"}}
\end{center}

\setcounter{section}{0}
\setcounter{table}{0}
\setcounter{figure}{0}

In this supplementary material, we provide more experiments, discussions, and other details that could not be included in the main text due to the lack of pages.
The contents are summarized below:
\begin{compactitem}
    \item Sec.~\ref{sec:co_registration_smplx}: Details of co-registration of SMPL-X
    \item Sec.~\ref{sec:mlp_architecture}: Detailed architecture of MLPs
    \item Sec.~\ref{sec:regularizers}: Regularizers
    \item Sec.~\ref{sec:running_time_compare}: Running time comparison
    \item Sec.~\ref{sec:geometry_comparison}: 3D geometry comparison
    \item Sec.~\ref{sec:compare_to_gen_ai}: Comparison to generative AIs
    \item Sec.~\ref{sec:implementation_details}: Implementation details
    \item Sec.~\ref{sec:failure_cases}: Failure cases
\end{compactitem}

\input{src_suppl/co_registration_smplx}
\input{src_suppl/mlp_architecture}
\input{src_suppl/regularizers}
\input{src_suppl/running_time_comparison}
\input{src_suppl/geometry_comparison}
\input{src_suppl/comparison_to_gen_ai}
\input{src_suppl/implementation_details} 
\input{src_suppl/failure_cases}
