# Supplementary material for: HOIGS: Human-Object Interaction Gaussian Splatting
Source: arXiv:2604.04016 source file (2026-04-05)
Supplement: Supplementary file 2 [file Appendix_HOINetwork.tex]

\begin{figure*}[t!]
\centerline{\includegraphics[width=0.6\textwidth]{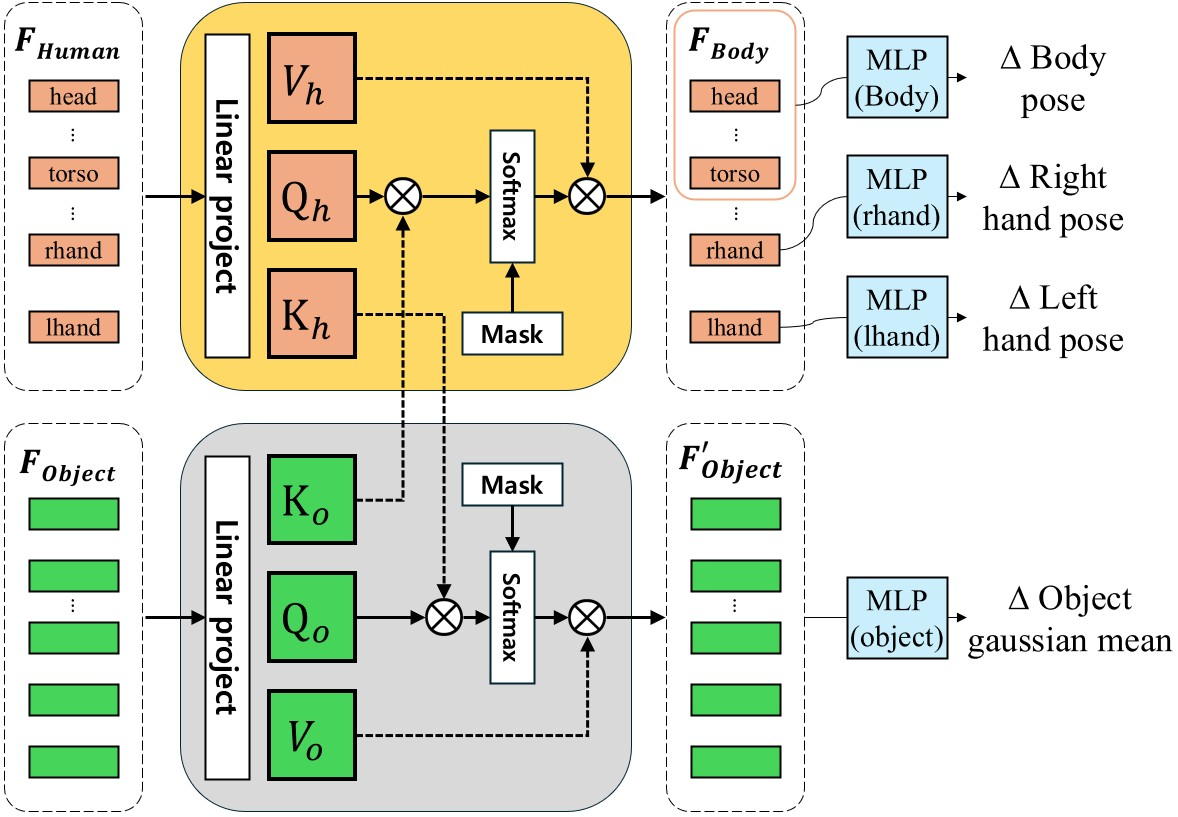}}
    \vspace{-2mm}
    \caption{\textbf{Detailed HOI network.}
    The proposed architecture for estimating human-object interactions, leveraging features from human body parts and object Gaussian representations. The model takes as input human part features and per-Gaussian object features, processes them through bidirectional attention mechanisms to incorporate mutual contextual information, and outputs predictions for SMPL-X parameters per body part along with offset adjustments for object Gaussian centers.}
    \label{appendix_HOINetwork}
    \vspace{-5mm}
\end{figure*}
