# Supplementary material for: HOIGS: Human-Object Interaction Gaussian Splatting
Source: arXiv:2604.04016 source file (2026-04-05)
Supplement: Supplementary file 3 [file Appendix_More_qualitative.tex]

\begin{figure*}[htb!]
\centerline{\includegraphics[width=\textwidth]{images/appendix/Appendix_1.png}}
    \vspace{-2mm}
    \caption{\textbf{Decomposed scene reconstruction.}
    Visualization of individual scene components demonstrating geometric integrity in occluded regions. From left to right: human-only rendering, object-only rendering, full scene rendering, and ground truth. Each row shows a different frame from the sequence, highlighting that both human and object maintain coherent geometry even during close contact and occlusion.}
    \label{fig:decomposed_render}
\end{figure*}
