# Supplementary material for: HOIGS: Human-Object Interaction Gaussian Splatting
Source: arXiv:2604.04016 source file (2026-04-05)
Supplement: Supplementary file 4 [file Appendix_More_qualitative1.tex]

\begin{figure*}[htb!]
\centerline{\includegraphics[width=\textwidth]{images/appendix/behave_refine.png}}
    \vspace{-2mm}
    \caption{\textbf{Qualitative comparison of human pose refinement on the BEHAVE dataset.}
    Visual comparison between ExAvatar and our method (HOIGS). The red boxes highlight the interaction regions (hands and objects). Our HOI module explicitly refines the hand and forearm poses by leveraging object motion features, leading to accurate contact modeling, whereas ExAvatar exhibits misalignment in these interaction-rich regions.}
    \label{appendix_behave_refine}
\end{figure*}
