# Supplementary material for: HOIGS: Human-Object Interaction Gaussian Splatting
Source: arXiv:2604.04016 source file (2026-04-05)
Supplement: Supplementary file 7 [file Appendix_human_feature.tex]

\begin{figure*}[t!]
\centerline{\includegraphics[width=\textwidth]{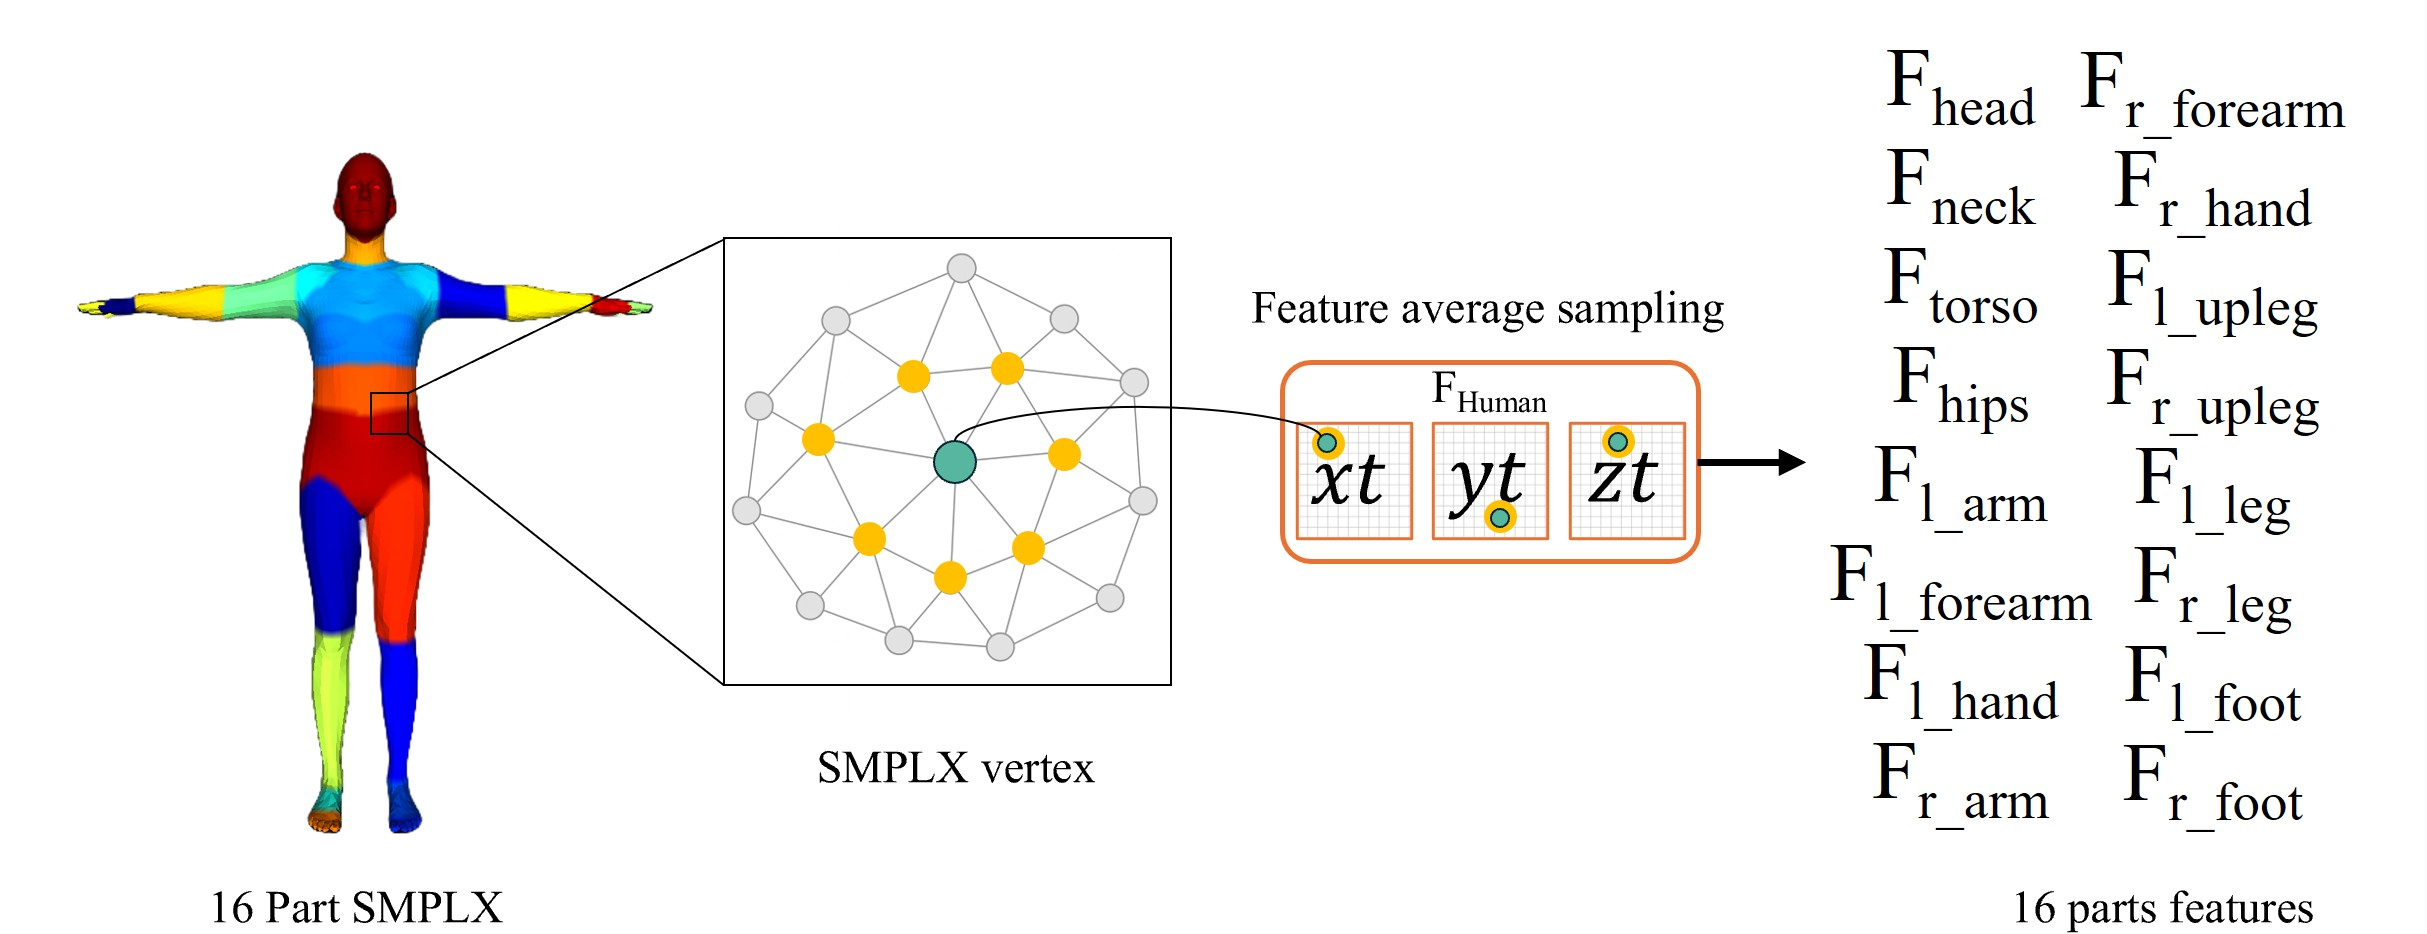}}
    \vspace{-2mm}
    \caption{\textbf{Human feature extraction.}
    }
    \label{appendix_humanfeature}
    \vspace{-5mm}
\end{figure*}
