# Supplementary material for: HOIGS: Human-Object Interaction Gaussian Splatting
Source: arXiv:2604.04016 source file (2026-04-05)
Supplement: Supplementary file 8 [file Appendix_BEHAVE.tex]

\begin{table*}[t]
\centering
\scriptsize
\caption{
Unified quantitative evaluation on the BEHAVE dataset. The values in each cell correspond to \textbf{PA-MPJPE / PA-MPJPE (Hand/Forearm) / PA-PVE}. HOIGS consistently outperforms the baseline across these metrics, particularly in interaction-critical regions.
}
\label{tab:unified_comparison}
\setlength\tabcolsep{1.0pt}

\resizebox{\textwidth}{!}{%
\begin{tabular}{C{2.5cm}|C{3.2cm}C{3.2cm}C{3.2cm}C{3.2cm}}
\specialrule{.1em}{.05em}{.05em}

% -------- Part 1: First 4 Classes --------
\textbf{Model} &
\textbf{Backpack\_1} &
\textbf{Plasticcontainer\_1} &
\textbf{Plasticcontainer\_2} &
\textbf{Suitcase\_2} \\ \hline

ExAvatar & 
0.4196 / 0.4628 / 0.3687 & 
0.3875 / 0.4282 / 0.3563 & 
0.3094 / 0.3145 / 0.2897 & 
0.2654 / 0.2957 / 0.2505 \\

HOIGS (Ours) & 
0.4177 / 0.4539 / 0.3656 & 
0.2964 / 0.3344 / 0.2863 & 
0.2973 / 0.3120 / 0.2837 & 
0.2438 / 0.2649 / 0.2352 \\

\specialrule{.1em}{.05em}{.05em}

% -------- Part 2: Next 4 Classes --------
\textbf{Model} &
\textbf{Backpack\_3} &
\textbf{Plasticcontainer\_3} &
\textbf{Backpack\_6} &
\textbf{Trashbin\_6} \\ \hline

ExAvatar & 
0.2690 / 0.3135 / 0.2488 & 
0.3293 / 0.3298 / 0.2970 & 
0.2177 / 0.2494 / 0.2092 & 
0.2294 / 0.2597 / 0.2156 \\

HOIGS (Ours) & 
0.2629 / 0.3068 / 0.2438 & 
0.3270 / 0.3265 / 0.2948 & 
0.2110 / 0.2380 / 0.2020 & 
0.2263 / 0.2550 / 0.2126 \\

\specialrule{.1em}{.05em}{.05em}

\end{tabular}%
}

\vspace{2mm}
\end{table*}
