# Supplementary material for: HOIGS: Human-Object Interaction Gaussian Splatting
Source: arXiv:2604.04016 source file (2026-04-05)
Supplement: Supplementary file 9 [file Appendix_BEHAVE2.tex]

\begin{table*}[t]
\centering
\caption{
Specific analysis for Hand and Forearm joints, which are the most critical regions for interaction tasks. We observe a larger performance gain in this metric compared to full-body evaluation. This indicates that the HOI module effectively refines the poses of interaction-related body parts through mutual feedback.
}
\label{tab:PA_MPJPE_hand_forearm}
\tiny
\setlength\tabcolsep{1.0pt}

\resizebox{\textwidth}{!}{%
\begin{tabular}{C{3.0cm}|C{2.5cm}C{2.5cm}C{2.5cm}C{2.5cm}}
\specialrule{.1em}{.05em}{.05em}

% -------- Part 1: First 4 Classes --------
\textbf{Model} &
\textbf{Backpack1} &
\textbf{Plasticcontainer1} &
\textbf{Plasticcontainer2} &
\textbf{Suitcase1} \\ \hline

ExAvatar & 
0.4628 & 
0.4282 & 
0.3145 & 
0.2957 \\

HOIGS (Ours) & 
0.4539 & 
0.3344 & 
0.3120 & 
0.2649 \\

\specialrule{.1em}{.05em}{.05em}

% -------- Part 2: Next 4 Classes --------
\textbf{Model} &
\textbf{Backpack2} &
\textbf{Plasticcontainer3} &
\textbf{Backpack3} &
\textbf{Trashbin} \\ \hline

ExAvatar & 
0.3135 & 
0.3298 & 
0.2494 & 
0.2597 \\

HOIGS (Ours) & 
0.3068 & 
0.3265 & 
0.2380 & 
0.2550 \\

\specialrule{.1em}{.05em}{.05em}

\end{tabular}%
}
\end{table*}
