# Supplementary material for: HOIGS: Human-Object Interaction Gaussian Splatting
Source: arXiv:2604.04016 source file (2026-04-05)
Supplement: Supplementary file 10 [file Appendix_BEHAVE3.tex]

\begin{table*}[t]
\centering
\caption{
Unified quantitative evaluation on the BEHAVE dataset. The values in each cell correspond to \textbf{PA-MPJPE / PA-MPJPE (Hand/Forearm) / PA-PVE}. HOIGS consistently outperforms the baseline across these metrics, particularly in interaction-critical regions.
}
\label{tab:unified_comparison}
\tiny
\setlength\tabcolsep{1.0pt}
 % Increased slightly for better separation of slashed values
\resizebox{\textwidth}{!}{%
\begin{tabular}{C{2.5cm}|C{3.2cm}C{3.2cm}C{3.2cm}C{3.2cm}}
\specialrule{.1em}{.05em}{.05em}

% -------- Part 1: First 4 Classes --------
\textbf{Model} &
\textbf{Backpack1} &
\textbf{Plasticcontainer1} &
\textbf{Plasticcontainer2} &
\textbf{Suitcase1} \\ \hline

ExAvatar & 
0.333 / 0.33 / 0.333 & 
0.333 / 0.33 / 0.333 & 
0.333 / 0.33 / 0.333 & 
0.333 / 0.33 / 0.333 \\

HOIGS (Ours) & 
0.333 / 0.33 / 0.333 & 
0.333 / 0.33 / 0.333 & 
0.333 / 0.33 / 0.333 & 
0.333 / 0.33 / 0.333 \\

\specialrule{.1em}{.05em}{.05em}

% -------- Part 2: Next 4 Classes --------
\textbf{Model} &
\textbf{Backpack2} &
\textbf{Plasticcontainer3} &
\textbf{Backpack3} &
\textbf{Trashbin} \\ \hline

ExAvatar & 
0.333 / 0.33 / 0.333 & 
0.333 / 0.33 / 0.333 & 
0.333 / 0.33 / 0.333 & 
0.333 / 0.33 / 0.333 \\

HOIGS (Ours) & 
0.333 / 0.33 / 0.333 & 
0.333 / 0.33 / 0.333 & 
0.333 / 0.33 / 0.333 & 
0.333 / 0.33 / 0.333 \\

\specialrule{.1em}{.05em}{.05em}

\end{tabular}%
}
\end{table*}
